# Supplementary material for: Long-range states and Feshbach resonances in collisions between ultracold alkali-metal diatomic molecules and atoms
Source: arXiv:2212.08030 ancillary file (2023-03-10)
Supplement: Supplementary file 1 [file Supplemental.pdf]

# Supplemental Material for Long-range states and Feshbach resonances in collisions between ultracold alkali-metal diatomic molecules and atoms

Matthew D. Frye and Jeremy M. Hutson

*Joint Quantum Centre (JQC) Durham-Newcastle, Department of Chemistry,  
Durham University, South Road, Durham DH1 3LE, United Kingdom*

(Dated: February 27, 2023)

Level crossing diagrams for  $\text{KRb}+\text{Rb}$  are shown in Figs. 1, 2, and 3 for  $a = 0$ ,  $\bar{a}$ , and  $2\bar{a}$ , respectively. These are directly equivalent to Fig. 3 of the main paper, which is shown for  $a = \infty$ . Tables I, II, III, and IV give tabulations of fields and quantum numbers for the states

crossing thresholds, corresponding to Fig. 3 of the main paper, and Figs. 1, 2, and 3, respectively. Tabulation of resonances is limited to resonances with  $B^{\text{res}} \leq 1200$  G and  $(n^{\text{res}} = 0, N^{\text{res}} \leq 2)$  or  $(n^{\text{res}} \leq 0, N^{\text{res}} = 0)$ .

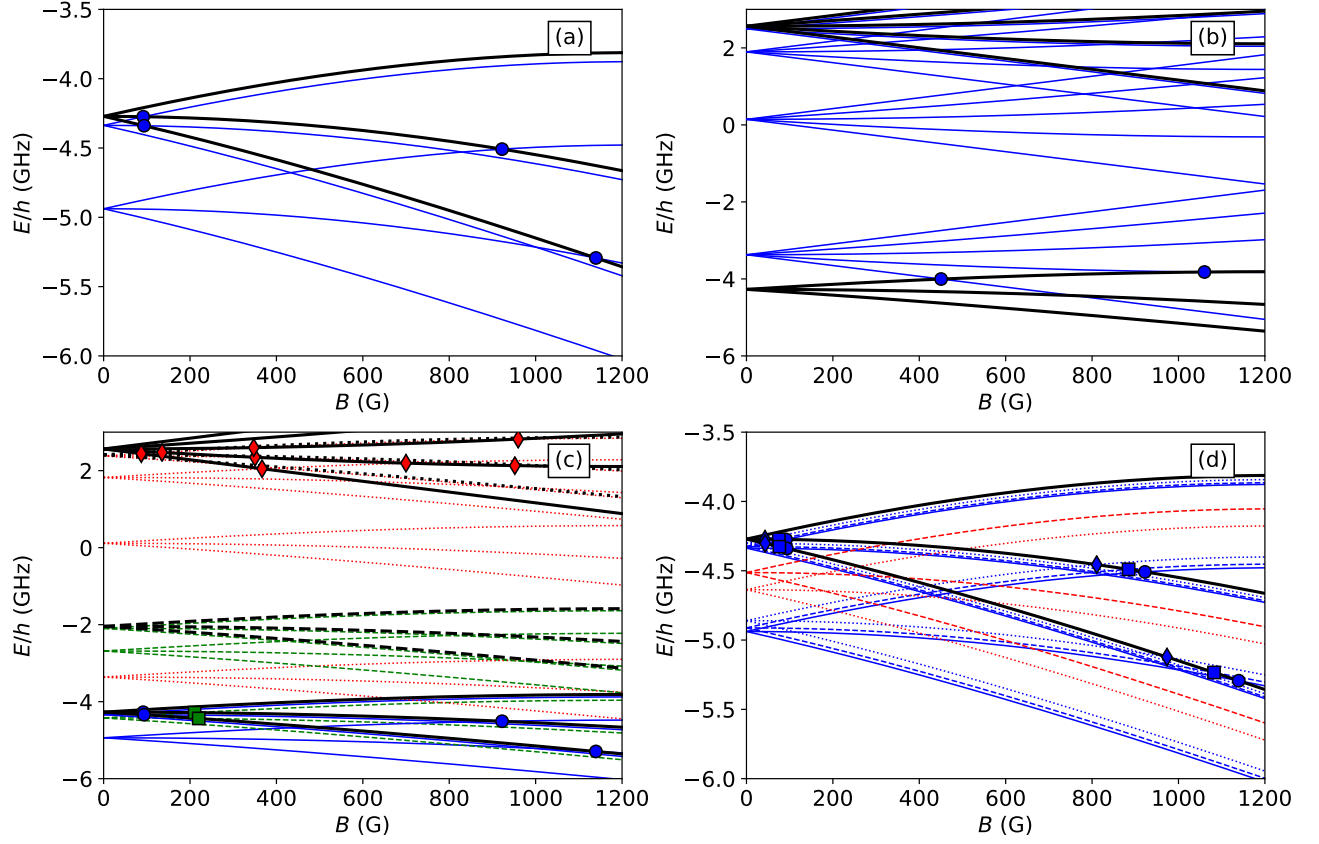

FIG. 1. Example level crossing diagram, equivalent to Fig. 3 of the main paper but with  $a = 0$ . Heavy black lines show thresholds, and thin colored lines show bound states. Crossings that can cause Feshbach resonances are marked by symbols. (a) States  $(n^{\text{res}}, \tilde{f}_C^{\text{res}}, L^{\text{res}}) = (0, 1, 0)$ . (b) States  $(0, 2, 0)$ . (c) States  $(0, 1, 0)$  are shown with blue solid lines and circles,  $(1, 1, 1)$  with green dashed lines and squares, and  $(2, 1, 2)$  with red dotted lines and diamonds. (d) States  $(0, 1, 0)$  are shown with solid lines and circles,  $(0, 1, 1)$  with dashed lines and squares, and  $(0, 1, 2)$  with dotted lines and diamonds. Also shown in red are the bottom of the bins for  $L^{\text{res}} = 1$  and 2.

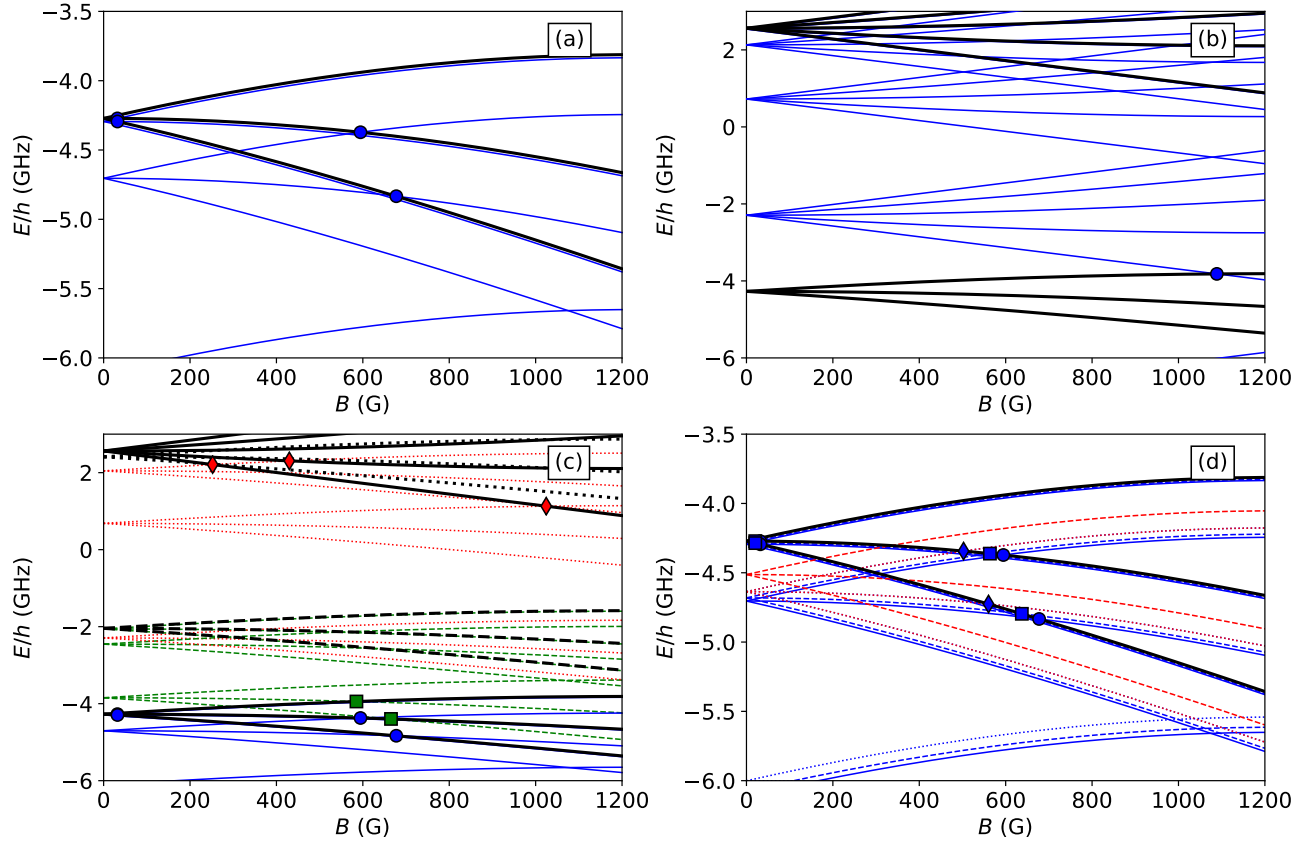

FIG. 2. Example level crossing diagram, equivalent to Fig. 3 of the main paper but with  $a = \bar{a}$ . Heavy black lines show thresholds, and thin colored lines show bound states. Crossings that can cause Feshbach resonances are marked by symbols. (a) States  $(n^{\text{res}}, \tilde{f}_C^{\text{res}}, L^{\text{res}}) = (0, 1, 0)$ . (b) States  $(0, 2, 0)$ . (c) States  $(0, 1, 0)$  are shown with blue solid lines and circles,  $(1, 1, 1)$  with green dashed lines and squares, and  $(2, 1, 2)$  with red dotted lines and diamonds. (d) States  $(0, 1, 0)$  are shown with solid lines and circles,  $(0, 1, 1)$  with dashed lines and squares, and  $(0, 1, 2)$  with dotted lines and diamonds. Also shown in red are the bottom of the bins for  $L^{\text{res}} = 1$  and 2.

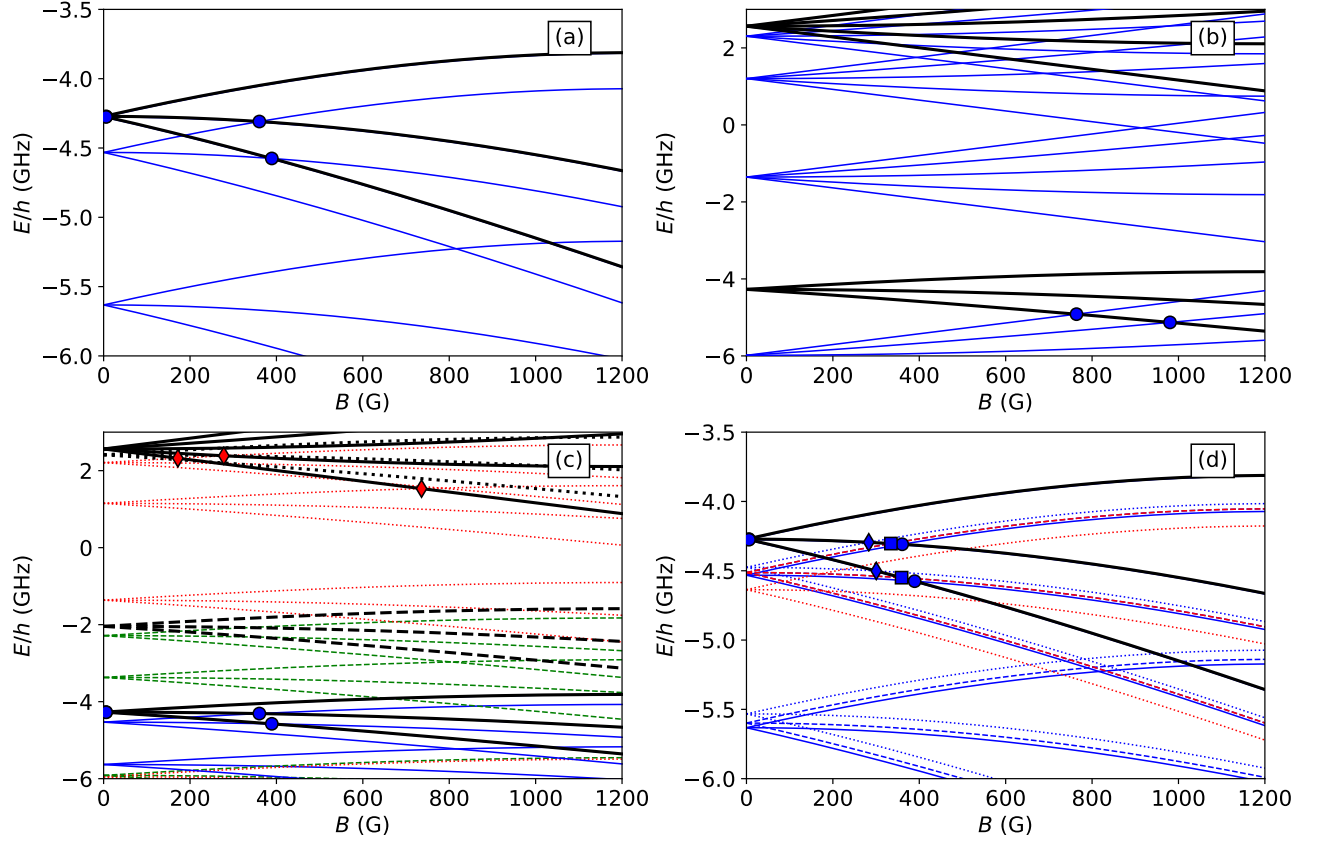

FIG. 3. Example level crossing diagram, equivalent to Fig. 3 of the main paper but with  $a = 2\bar{a}$ . Heavy black lines show thresholds, and thin colored lines show bound states. Crossings that can cause Feshbach resonances are marked by symbols. (a) States  $(n^{\text{res}}, \tilde{f}_C^{\text{res}}, L^{\text{res}}) = (0, 1, 0)$ . (b) States  $(0, 2, 0)$ . (c) States  $(0, 1, 0)$  are shown with blue solid lines and circles,  $(1, 1, 1)$  with green dashed lines and squares, and  $(2, 1, 2)$  with red dotted lines and diamonds. (d) States  $(0, 1, 0)$  are shown with solid lines and circles,  $(0, 1, 1)$  with dashed lines and squares, and  $(0, 1, 2)$  with dotted lines and diamonds. Also shown in red are the bottom of the bins for  $L^{\text{res}} = 1$  and 2.

TABLE I. Tabulation of calculated resonance positions along with bound-state quantum numbers for  $a = \infty$ .

|    | $\tilde{f}_{\text{Rb}}^{\text{in}}$ | $m_{f,\text{Rb}}^{\text{in}}$ | $\tilde{f}_{\text{Rb}}^{\text{res}}$ | $m_{f,\text{Rb}}^{\text{res}}$ | $n^{\text{res}}$ | $L^{\text{res}}$ | $N_{\text{min}}^{\text{res}}$ | $\eta$ | $B^{\text{res}}$ (G) |
|----|-------------------------------------|-------------------------------|--------------------------------------|--------------------------------|------------------|------------------|-------------------------------|--------|----------------------|
| 1  | 1                                   | 1                             | 1                                    | 0                              | 0                | 0                | 0                             | -1     | 202.1                |
| 2  | 1                                   | 1                             | 2                                    | 0                              | 0                | 0                | 0                             | -4     | 340.1                |
| 3  | 1                                   | 1                             | 2                                    | 1                              | 0                | 0                | 0                             | -4     | 198.9                |
| 4  | 1                                   | 1                             | 2                                    | 2                              | 0                | 0                | 0                             | -4     | 138.5                |
| 5  | 1                                   | 0                             | 1                                    | -1                             | 0                | 0                | 0                             | -1     | 194.1                |
| 6  | 1                                   | 0                             | 2                                    | 0                              | 0                | 0                | 0                             | -4     | 724.2                |
| 7  | 1                                   | 0                             | 2                                    | 1                              | 0                | 0                | 0                             | -4     | 341.0                |
| 8  | 2                                   | -2                            | 2                                    | -1                             | 0                | 0                | 0                             | -1     | 187.0                |
| 9  | 2                                   | -2                            | 2                                    | -1                             | 0                | 0                | 0                             | -2     | 1004.4               |
| 10 | 2                                   | -1                            | 2                                    | 0                              | 0                | 0                | 0                             | -1     | 194.8                |
| 11 | 2                                   | 0                             | 2                                    | 1                              | 0                | 0                | 0                             | -1     | 202.9                |
| 12 | 2                                   | 1                             | 2                                    | 2                              | 0                | 0                | 0                             | -1     | 211.4                |
| 13 | 1                                   | 1                             | 1                                    | 0                              | 0                | 1                | 1                             | -1     | 179.0                |
| 14 | 1                                   | 1                             | 2                                    | 0                              | 0                | 1                | 1                             | -4     | 282.2                |
| 15 | 1                                   | 1                             | 2                                    | 1                              | 0                | 1                | 1                             | -4     | 161.5                |
| 16 | 1                                   | 1                             | 2                                    | 2                              | 0                | 1                | 1                             | -4     | 111.6                |
| 17 | 1                                   | 0                             | 1                                    | -1                             | 0                | 1                | 1                             | -1     | 172.7                |
| 18 | 1                                   | 0                             | 2                                    | 0                              | 0                | 1                | 1                             | -4     | 647.8                |
| 19 | 1                                   | 0                             | 2                                    | 1                              | 0                | 1                | 1                             | -4     | 283.0                |
| 20 | 2                                   | -2                            | 2                                    | -1                             | 0                | 1                | 1                             | -1     | 167.2                |
| 21 | 2                                   | -2                            | 2                                    | -1                             | 0                | 1                | 1                             | -2     | 980.7                |
| 22 | 2                                   | -1                            | 2                                    | 0                              | 0                | 1                | 1                             | -1     | 173.3                |
| 23 | 2                                   | 0                             | 2                                    | 1                              | 0                | 1                | 1                             | -1     | 179.8                |
| 24 | 2                                   | 1                             | 2                                    | 2                              | 0                | 1                | 1                             | -1     | 186.4                |
| 25 | 1                                   | 1                             | 1                                    | 0                              | 0                | 2                | 2                             | -1     | 134.5                |
| 26 | 1                                   | 1                             | 2                                    | 0                              | 0                | 2                | 2                             | -4     | 155.8                |
| 27 | 1                                   | 1                             | 2                                    | 1                              | 0                | 2                | 2                             | -4     | 84.5                 |
| 28 | 1                                   | 1                             | 2                                    | 2                              | 0                | 2                | 2                             | -4     | 57.4                 |
| 29 | 1                                   | 0                             | 1                                    | -1                             | 0                | 2                | 2                             | -1     | 130.9                |
| 30 | 1                                   | 0                             | 2                                    | 0                              | 0                | 2                | 2                             | -4     | 461.7                |
| 31 | 1                                   | 0                             | 2                                    | 1                              | 0                | 2                | 2                             | -4     | 156.3                |
| 32 | 2                                   | -2                            | 2                                    | -1                             | 0                | 2                | 2                             | -1     | 127.9                |
| 33 | 2                                   | -2                            | 2                                    | -1                             | 0                | 2                | 2                             | -2     | 932.6                |
| 34 | 2                                   | -1                            | 2                                    | 0                              | 0                | 2                | 2                             | -1     | 131.4                |
| 35 | 2                                   | 0                             | 2                                    | 1                              | 0                | 2                | 2                             | -1     | 135.1                |
| 36 | 2                                   | 1                             | 2                                    | 2                              | 0                | 2                | 2                             | -1     | 138.8                |
| 37 | 1                                   | 0                             | 1                                    | -1                             | 1                | 1                | 0                             | -3     | 1148.9               |
| 38 | 1                                   | -1                            | 2                                    | -2                             | 1                | 1                | 0                             | -4     | 1097.7               |
| 39 | 2                                   | -2                            | 2                                    | -1                             | 1                | 1                | 0                             | -3     | 884.9                |
| 40 | 2                                   | -1                            | 2                                    | 0                              | 1                | 1                | 0                             | -3     | 1153.9               |
| 41 | 1                                   | 1                             | 1                                    | 0                              | 2                | 2                | 0                             | -4     | 409.2                |
| 42 | 1                                   | 0                             | 1                                    | -1                             | 2                | 2                | 0                             | -4     | 377.5                |
| 43 | 1                                   | 0                             | 2                                    | -1                             | 2                | 2                | 0                             | -5     | 54.4                 |
| 44 | 1                                   | -1                            | 2                                    | -2                             | 2                | 2                | 0                             | -5     | 17.4                 |
| 45 | 1                                   | -1                            | 2                                    | -1                             | 2                | 2                | 0                             | -5     | 26.3                 |
| 46 | 1                                   | -1                            | 2                                    | 0                              | 2                | 2                | 0                             | -5     | 54.2                 |
| 47 | 2                                   | -2                            | 1                                    | -1                             | 2                | 2                | 0                             | -1     | 117.7                |
| 48 | 2                                   | -2                            | 1                                    | -1                             | 2                | 2                | 0                             | -2     | 519.2                |
| 49 | 2                                   | -2                            | 2                                    | -1                             | 2                | 2                | 0                             | -4     | 349.5                |
| 50 | 2                                   | -1                            | 1                                    | -1                             | 2                | 2                | 0                             | -1     | 185.2                |
| 51 | 2                                   | -1                            | 2                                    | 0                              | 2                | 2                | 0                             | -4     | 379.0                |
| 52 | 2                                   | 0                             | 2                                    | 1                              | 2                | 2                | 0                             | -4     | 411.1                |
| 53 | 2                                   | 1                             | 2                                    | 2                              | 2                | 2                | 0                             | -4     | 445.8                |

TABLE II. Tabulation of calculated resonance positions along with bound-state quantum numbers for  $a = 0$ .

|    | $\tilde{f}_{\text{Rb}}^{\text{in}}$ | $m_{f,\text{Rb}}^{\text{in}}$ | $\tilde{f}_{\text{Rb}}^{\text{res}}$ | $m_{f,\text{Rb}}^{\text{res}}$ | $n^{\text{res}}$ | $L^{\text{res}}$ | $N_{\text{min}}^{\text{res}}$ | $\eta$ | $B^{\text{res}}$ (G) |
|----|-------------------------------------|-------------------------------|--------------------------------------|--------------------------------|------------------|------------------|-------------------------------|--------|----------------------|
| 1  | 1                                   | 1                             | 1                                    | 0                              | 0                | 0                | 0                             | -1     | 93.5                 |
| 2  | 1                                   | 1                             | 1                                    | 0                              | 0                | 0                | 0                             | -2     | 1139.5               |
| 3  | 1                                   | 0                             | 1                                    | -1                             | 0                | 0                | 0                             | -1     | 91.7                 |
| 4  | 1                                   | 0                             | 1                                    | -1                             | 0                | 0                | 0                             | -2     | 922.3                |
| 5  | 1                                   | -1                            | 2                                    | -2                             | 0                | 0                | 0                             | -4     | 450.5                |
| 6  | 1                                   | -1                            | 2                                    | -1                             | 0                | 0                | 0                             | -4     | 1060.2               |
| 7  | 2                                   | -2                            | 2                                    | -1                             | 0                | 0                | 0                             | -1     | 90.3                 |
| 8  | 2                                   | -2                            | 2                                    | -1                             | 0                | 0                | 0                             | -2     | 751.7                |
| 9  | 2                                   | -1                            | 2                                    | 0                              | 0                | 0                | 0                             | -1     | 92.1                 |
| 10 | 2                                   | -1                            | 2                                    | 0                              | 0                | 0                | 0                             | -2     | 926.1                |
| 11 | 2                                   | 0                             | 2                                    | 1                              | 0                | 0                | 0                             | -1     | 93.8                 |
| 12 | 2                                   | 0                             | 2                                    | 1                              | 0                | 0                | 0                             | -2     | 1146.5               |
| 13 | 2                                   | 1                             | 2                                    | 2                              | 0                | 0                | 0                             | -1     | 95.7                 |
| 14 | 1                                   | 1                             | 1                                    | 0                              | 0                | 1                | 1                             | -1     | 76.1                 |
| 15 | 1                                   | 1                             | 1                                    | 0                              | 0                | 1                | 1                             | -2     | 1082.2               |
| 16 | 1                                   | 0                             | 1                                    | -1                             | 0                | 1                | 1                             | -1     | 75.0                 |
| 17 | 1                                   | 0                             | 1                                    | -1                             | 0                | 1                | 1                             | -2     | 884.6                |
| 18 | 1                                   | -1                            | 2                                    | -2                             | 0                | 1                | 1                             | -4     | 479.7                |
| 19 | 2                                   | -2                            | 2                                    | -1                             | 0                | 1                | 1                             | -1     | 74.1                 |
| 20 | 2                                   | -2                            | 2                                    | -1                             | 0                | 1                | 1                             | -2     | 727.6                |
| 21 | 2                                   | -1                            | 2                                    | 0                              | 0                | 1                | 1                             | -1     | 75.3                 |
| 22 | 2                                   | -1                            | 2                                    | 0                              | 0                | 1                | 1                             | -2     | 888.1                |
| 23 | 2                                   | 0                             | 2                                    | 1                              | 0                | 1                | 1                             | -1     | 76.4                 |
| 24 | 2                                   | 0                             | 2                                    | 1                              | 0                | 1                | 1                             | -2     | 1088.8               |
| 25 | 2                                   | 1                             | 2                                    | 2                              | 0                | 1                | 1                             | -1     | 77.6                 |
| 26 | 1                                   | 1                             | 1                                    | 0                              | 0                | 2                | 2                             | -1     | 43.3                 |
| 27 | 1                                   | 1                             | 1                                    | 0                              | 0                | 2                | 2                             | -2     | 973.4                |
| 28 | 1                                   | 0                             | 1                                    | -1                             | 0                | 2                | 2                             | -1     | 43.0                 |
| 29 | 1                                   | 0                             | 1                                    | -1                             | 0                | 2                | 2                             | -2     | 810.7                |
| 30 | 1                                   | -1                            | 2                                    | -2                             | 0                | 2                | 2                             | -4     | 538.6                |
| 31 | 2                                   | -2                            | 2                                    | -1                             | 0                | 2                | 2                             | -1     | 42.7                 |
| 32 | 2                                   | -2                            | 2                                    | -1                             | 0                | 2                | 2                             | -2     | 678.9                |
| 33 | 2                                   | -1                            | 2                                    | 0                              | 0                | 2                | 2                             | -1     | 43.1                 |
| 34 | 2                                   | -1                            | 2                                    | 0                              | 0                | 2                | 2                             | -2     | 813.9                |
| 35 | 2                                   | 0                             | 2                                    | 1                              | 0                | 2                | 2                             | -1     | 43.5                 |
| 36 | 2                                   | 0                             | 2                                    | 1                              | 0                | 2                | 2                             | -2     | 979.0                |
| 37 | 2                                   | 1                             | 2                                    | 2                              | 0                | 2                | 2                             | -1     | 43.9                 |
| 38 | 2                                   | 1                             | 2                                    | 2                              | 0                | 2                | 2                             | -2     | 1174.3               |
| 39 | 1                                   | 1                             | 1                                    | 0                              | 1                | 1                | 0                             | -3     | 220.1                |
| 40 | 1                                   | 1                             | 2                                    | 2                              | 1                | 1                | 0                             | -5     | 1173.6               |
| 41 | 1                                   | 0                             | 1                                    | -1                             | 1                | 1                | 0                             | -3     | 210.6                |
| 42 | 2                                   | -2                            | 2                                    | -1                             | 1                | 1                | 0                             | -3     | 202.2                |
| 43 | 2                                   | -1                            | 2                                    | 0                              | 1                | 1                | 0                             | -3     | 211.4                |
| 44 | 2                                   | 0                             | 2                                    | 1                              | 1                | 1                | 0                             | -3     | 221.0                |
| 45 | 2                                   | 1                             | 2                                    | 2                              | 1                | 1                | 0                             | -3     | 231.0                |
| 46 | 1                                   | -1                            | 2                                    | -2                             | 2                | 2                | 0                             | -5     | 1033.0               |
| 47 | 2                                   | -2                            | 1                                    | -1                             | 2                | 2                | 0                             | -1     | 87.2                 |
| 48 | 2                                   | -2                            | 1                                    | -1                             | 2                | 2                | 0                             | -2     | 366.7                |
| 49 | 2                                   | -1                            | 1                                    | 0                              | 2                | 2                | 0                             | -1     | 350.4                |
| 50 | 2                                   | -1                            | 1                                    | 0                              | 2                | 2                | 0                             | -1     | 951.9                |
| 51 | 2                                   | -1                            | 1                                    | -1                             | 2                | 2                | 0                             | -1     | 135.3                |
| 52 | 2                                   | -1                            | 1                                    | -1                             | 2                | 2                | 0                             | -2     | 699.9                |
| 53 | 2                                   | -1                            | 2                                    | -2                             | 2                | 2                | 0                             | -4     | 961.8                |
| 54 | 2                                   | 0                             | 1                                    | -1                             | 2                | 2                | 0                             | -1     | 347.5                |
| 55 | 2                                   | 0                             | 1                                    | -1                             | 2                | 2                | 0                             | -1     | 959.7                |

TABLE III. Tabulation of calculated resonance positions along with bound-state quantum numbers for  $a = \bar{a}$ .

|    | $\tilde{f}_{\text{Rb}}^{\text{in}}$ | $m_{f,\text{Rb}}^{\text{in}}$ | $\tilde{f}_{\text{Rb}}^{\text{res}}$ | $m_{f,\text{Rb}}^{\text{res}}$ | $n^{\text{res}}$ | $L^{\text{res}}$ | $N_{\text{min}}^{\text{res}}$ | $\eta$ | $B^{\text{res}}$ (G) |
|----|-------------------------------------|-------------------------------|--------------------------------------|--------------------------------|------------------|------------------|-------------------------------|--------|----------------------|
| 1  | 1                                   | 1                             | 1                                    | 0                              | 0                | 0                | 0                             | -1     | 32.1                 |
| 2  | 1                                   | 1                             | 1                                    | 0                              | 0                | 0                | 0                             | -2     | 677.4                |
| 3  | 1                                   | 0                             | 1                                    | -1                             | 0                | 0                | 0                             | -1     | 31.9                 |
| 4  | 1                                   | 0                             | 1                                    | -1                             | 0                | 0                | 0                             | -2     | 594.6                |
| 5  | 1                                   | -1                            | 2                                    | -2                             | 0                | 0                | 0                             | -4     | 1088.8               |
| 6  | 2                                   | -2                            | 2                                    | -1                             | 0                | 0                | 0                             | -1     | 31.8                 |
| 7  | 2                                   | -2                            | 2                                    | -1                             | 0                | 0                | 0                             | -2     | 524.0                |
| 8  | 2                                   | -1                            | 2                                    | 0                              | 0                | 0                | 0                             | -1     | 32.0                 |
| 9  | 2                                   | -1                            | 2                                    | 0                              | 0                | 0                | 0                             | -2     | 596.9                |
| 10 | 2                                   | 0                             | 2                                    | 1                              | 0                | 0                | 0                             | -1     | 32.3                 |
| 11 | 2                                   | 0                             | 2                                    | 1                              | 0                | 0                | 0                             | -2     | 680.8                |
| 12 | 2                                   | 1                             | 2                                    | 2                              | 0                | 0                | 0                             | -1     | 32.5                 |
| 13 | 2                                   | 1                             | 2                                    | 2                              | 0                | 0                | 0                             | -2     | 775.7                |
| 14 | 1                                   | 1                             | 1                                    | 0                              | 0                | 1                | 1                             | -1     | 20.3                 |
| 15 | 1                                   | 1                             | 1                                    | 0                              | 0                | 1                | 1                             | -2     | 637.4                |
| 16 | 1                                   | 0                             | 1                                    | -1                             | 0                | 1                | 1                             | -1     | 20.2                 |
| 17 | 1                                   | 0                             | 1                                    | -1                             | 0                | 1                | 1                             | -2     | 563.6                |
| 18 | 1                                   | -1                            | 2                                    | -2                             | 0                | 1                | 1                             | -4     | 1123.4               |
| 19 | 2                                   | -2                            | 2                                    | -1                             | 0                | 1                | 1                             | -1     | 20.2                 |
| 20 | 2                                   | -2                            | 2                                    | -1                             | 0                | 1                | 1                             | -2     | 500.2                |
| 21 | 2                                   | -1                            | 2                                    | 0                              | 0                | 1                | 1                             | -1     | 20.3                 |
| 22 | 2                                   | -1                            | 2                                    | 0                              | 0                | 1                | 1                             | -2     | 565.7                |
| 23 | 2                                   | 0                             | 2                                    | 1                              | 0                | 1                | 1                             | -1     | 20.4                 |
| 24 | 2                                   | 0                             | 2                                    | 1                              | 0                | 1                | 1                             | -2     | 640.5                |
| 25 | 2                                   | 1                             | 2                                    | 2                              | 0                | 1                | 1                             | -1     | 20.5                 |
| 26 | 2                                   | 1                             | 2                                    | 2                              | 0                | 1                | 1                             | -2     | 724.6                |
| 27 | 1                                   | 1                             | 1                                    | 0                              | 0                | 2                | 2                             | -1     | 560.3                |
| 28 | 1                                   | 0                             | 1                                    | -1                             | 0                | 2                | 2                             | -1     | 502.5                |
| 29 | 1                                   | -1                            | 2                                    | -2                             | 0                | 2                | 2                             | -3     | 1194.1               |
| 30 | 2                                   | -2                            | 2                                    | -1                             | 0                | 2                | 2                             | -1     | 452.2                |
| 31 | 2                                   | -1                            | 2                                    | 0                              | 0                | 2                | 2                             | -1     | 504.4                |
| 32 | 2                                   | 0                             | 2                                    | 1                              | 0                | 2                | 2                             | -1     | 562.9                |
| 33 | 2                                   | 1                             | 2                                    | 2                              | 0                | 2                | 2                             | -1     | 627.9                |
| 34 | 1                                   | 1                             | 2                                    | 0                              | 1                | 1                | 0                             | -5     | 879.6                |
| 35 | 1                                   | 1                             | 2                                    | 1                              | 1                | 1                | 0                             | -5     | 596.8                |
| 36 | 1                                   | 1                             | 2                                    | 2                              | 1                | 1                | 0                             | -5     | 444.3                |
| 37 | 1                                   | 0                             | 1                                    | 1                              | 1                | 1                | 0                             | -3     | 665.2                |
| 38 | 1                                   | 0                             | 2                                    | 1                              | 1                | 1                | 0                             | -5     | 881.3                |
| 39 | 1                                   | -1                            | 1                                    | 0                              | 1                | 1                | 0                             | -3     | 585.2                |
| 40 | 2                                   | -1                            | 2                                    | -2                             | 1                | 1                | 0                             | -3     | 516.8                |
| 41 | 2                                   | 0                             | 2                                    | -1                             | 1                | 1                | 0                             | -3     | 587.4                |
| 42 | 2                                   | 1                             | 2                                    | 0                              | 1                | 1                | 0                             | -3     | 668.5                |
| 43 | 2                                   | 2                             | 2                                    | 1                              | 1                | 1                | 0                             | -3     | 760.0                |
| 44 | 2                                   | -2                            | 1                                    | -1                             | 2                | 2                | 0                             | -1     | 252.3                |
| 45 | 2                                   | -2                            | 1                                    | -1                             | 2                | 2                | 0                             | -2     | 1024.5               |
| 46 | 2                                   | -1                            | 1                                    | -1                             | 2                | 2                | 0                             | -1     | 429.9                |

TABLE IV. Tabulation of calculated resonance positions along with bound-state quantum numbers for  $a = 2\bar{a}$ .

|    | $\tilde{f}_{\text{Rb}}^{\text{in}}$ | $m_{f,\text{Rb}}^{\text{in}}$ | $\tilde{f}_{\text{Rb}}^{\text{res}}$ | $m_{f,\text{Rb}}^{\text{res}}$ | $n^{\text{res}}$ | $L^{\text{res}}$ | $N_{\text{min}}^{\text{res}}$ | $\eta$ | $B^{\text{res}}$ (G) |
|----|-------------------------------------|-------------------------------|--------------------------------------|--------------------------------|------------------|------------------|-------------------------------|--------|----------------------|
| 1  | 1                                   | 1                             | 1                                    | 0                              | 0                | 0                | 0                             | -1     | 5.7                  |
| 2  | 1                                   | 1                             | 1                                    | 0                              | 0                | 0                | 0                             | -2     | 389.3                |
| 3  | 1                                   | 1                             | 2                                    | 1                              | 0                | 0                | 0                             | -5     | 980.4                |
| 4  | 1                                   | 1                             | 2                                    | 2                              | 0                | 0                | 0                             | -5     | 763.9                |
| 5  | 1                                   | 0                             | 1                                    | -1                             | 0                | 0                | 0                             | -1     | 5.7                  |
| 6  | 1                                   | 0                             | 1                                    | -1                             | 0                | 0                | 0                             | -2     | 360.5                |
| 7  | 2                                   | -2                            | 2                                    | -1                             | 0                | 0                | 0                             | -1     | 5.7                  |
| 8  | 2                                   | -2                            | 2                                    | -1                             | 0                | 0                | 0                             | -2     | 335.0                |
| 9  | 2                                   | -1                            | 2                                    | 0                              | 0                | 0                | 0                             | -1     | 5.7                  |
| 10 | 2                                   | -1                            | 2                                    | 0                              | 0                | 0                | 0                             | -2     | 361.9                |
| 11 | 2                                   | 0                             | 2                                    | 1                              | 0                | 0                | 0                             | -1     | 5.7                  |
| 12 | 2                                   | 0                             | 2                                    | 1                              | 0                | 0                | 0                             | -2     | 391.0                |
| 13 | 2                                   | 1                             | 2                                    | 2                              | 0                | 0                | 0                             | -1     | 5.7                  |
| 14 | 2                                   | 1                             | 2                                    | 2                              | 0                | 0                | 0                             | -2     | 422.4                |
| 15 | 1                                   | 1                             | 1                                    | 0                              | 0                | 1                | 1                             | -1     | 359.1                |
| 16 | 1                                   | 1                             | 2                                    | 1                              | 0                | 1                | 1                             | -4     | 949.8                |
| 17 | 1                                   | 1                             | 2                                    | 2                              | 0                | 1                | 1                             | -4     | 737.7                |
| 18 | 1                                   | 0                             | 1                                    | -1                             | 0                | 1                | 1                             | -1     | 334.4                |
| 19 | 2                                   | -2                            | 2                                    | -1                             | 0                | 1                | 1                             | -1     | 312.6                |
| 20 | 2                                   | -1                            | 2                                    | 0                              | 0                | 1                | 1                             | -1     | 335.7                |
| 21 | 2                                   | 0                             | 2                                    | 1                              | 0                | 1                | 1                             | -1     | 360.6                |
| 22 | 2                                   | 1                             | 2                                    | 2                              | 0                | 1                | 1                             | -1     | 387.4                |
| 23 | 1                                   | 1                             | 1                                    | 0                              | 0                | 2                | 2                             | -1     | 300.5                |
| 24 | 1                                   | 1                             | 2                                    | 1                              | 0                | 2                | 2                             | -4     | 888.1                |
| 25 | 1                                   | 1                             | 2                                    | 2                              | 0                | 2                | 2                             | -4     | 685.3                |
| 26 | 1                                   | 0                             | 1                                    | -1                             | 0                | 2                | 2                             | -1     | 283.1                |
| 27 | 2                                   | -2                            | 2                                    | -1                             | 0                | 2                | 2                             | -1     | 267.6                |
| 28 | 2                                   | -1                            | 2                                    | 0                              | 0                | 2                | 2                             | -1     | 284.1                |
| 29 | 2                                   | 0                             | 2                                    | 1                              | 0                | 2                | 2                             | -1     | 301.8                |
| 30 | 2                                   | 1                             | 2                                    | 2                              | 0                | 2                | 2                             | -1     | 320.5                |
| 31 | 1                                   | -1                            | 2                                    | -2                             | 1                | 1                | 0                             | -4     | 283.1                |
| 32 | 1                                   | -1                            | 2                                    | -1                             | 1                | 1                | 0                             | -4     | 494.1                |
| 33 | 2                                   | -1                            | 2                                    | -2                             | 1                | 1                | 0                             | -2     | 953.3                |
| 34 | 1                                   | 1                             | 2                                    | 1                              | 2                | 2                | 0                             | -5     | 1176.0               |
| 35 | 1                                   | 1                             | 2                                    | 2                              | 2                | 2                | 0                             | -5     | 933.4                |
| 36 | 2                                   | -2                            | 1                                    | -1                             | 2                | 2                | 0                             | -1     | 171.9                |
| 37 | 2                                   | -2                            | 1                                    | -1                             | 2                | 2                | 0                             | -2     | 735.9                |
| 38 | 2                                   | -1                            | 1                                    | -1                             | 2                | 2                | 0                             | -1     | 278.2                |
